# Supplementary material for: Robust Vacuity for Branching Temporal Logic
Source: arXiv:1002.4616 source file (2010-10-13)
Supplement: Supplementary file 1 [file appendix.tex]

\section{Proofs of Select Theorems}

\setcounter{theorem}{10}

\begin{theorem}
  Let $K$ be a \kripke structure, and $K_x$ be as described in the beginning of Section~\ref{sec:vacu-detect-via-1}. Then,
  $K' \in \C(K_x)$ iff $K'$ is $\{x\}$-bisimilar to $K$.
\end{theorem}

\begin{Proof}
The proof follows
trivially from the definitions of $\{x\}$-bisimulation and refinement.
\end{Proof}

\begin{theorem}
  A formula $\varphi$ is $\psi$-vacuous in an abstract model
  $K_\alpha$ iff $\varphi[\psi \subst x]$ does not evaluate to \maybe in
  $(K_\alpha)_x$, under thorough semantics. %
\end{theorem}

\begin{Proof}
  For an atomic proposition $x$ of $K$, let $K_{-x}$ denote a \kripke
  structure constructed from $K$ by \emph{removing} $x$ from $K$; that
  is, $K = (K_x)_{-x}$. Note that both $K$ and $K_{-x}$ are defined
  over an identical set of states $S$. Furthermore, 
$(K_{-x})_x \infoleq K$ under the identity
  relation $id = \{(s,s) \mid s \in S\}$.
  
Refinements of $K_x$ are related to refinements
  of $K$: $K_x \infoleq K' \liff K \infoleq (K')_{-x}$ because $x$ is
  \maybe in every state of $K_x$, and the statespaces of $K_x$ and $K$
  are identical.  Thus, the set of
  concretizations of $K_x$ is equivalent to a set obtained by: (a)
  concretizing $K$, (b) adding the atomic proposition $x$, and (c) taking
  the concretization of the result, i.e. $\C(K_x) = \C((\C(K))_x)$.
  
  Finally, we prove the theorem.

\vspace{-0.1in}

  \[
  \begin{array}{ll}
       & ||\varphi[\psi \subst x]||_t^{(K_\alpha)_x} = \true\\
\liff  & \lhint{by Definition~\ref{def:thorough-semantics}}\\
       & \A{K \in \C((K_\alpha)_x)} ||\varphi[\psi \subst x]||^K = \true\\
\liff  & \lhint{since $\C(K_x) = \C((\C(K))_x)$}\\
      & \A{K \in \C(\C((K_\alpha))_x)} ||\varphi[\psi \subst x]||^K = \true\\ 
\liff  & \lhint{by Definition~\ref{def:thorough-semantics}}\\
       & \A{K \in \C(K_\alpha)} ||\varphi[\psi \subst x]||_t^{K_x} = \true\\ 
  \end{array}
  \]
  The proof of the second case is similar.
\end{Proof}
